# Supplementary material for: Better Late than Never; Scaling Computation in Blockchains by Delaying Execution
Source: arXiv:2005.11791 source file (2021-06-02)
Supplement: Supplementary file 1 [file hca-analysis.tex]

% !TEX root = ../main.tex
\section{Analysis of MAR and RAR}
\label{sec:hca analysis}
We compute an approximation to the fraction of late blocks for both
RAR and MAR using the Markov chain~(MC) shown in
Figure~\ref{fig:hidden chain mc}.  Our analysis neglects the
possibility of the honest queue equaling $\ths$ before $t$.  It
counts the late blocks when $A_{\advi}(t)>A_{\hsti}(t)$ and 
$A_{\advi}(t)\ge\ths$ and assumes that $Q(t)=A_{\advi}(t)$ when in 
fact $Q(t)\ge A_{\advi}(t)$. As a result this undercounts
the number of late blocks in this case.
 
A state $(x,y)$ represents that \adv 
has mined $y$ blocks in its hidden chain and honest miners have
created $x$ blocks, extending $B_i$. For example, state 
$(0,0)$ represents that, \adv has no blocks in its hidden
chain extending $B_i$ and honest miners also didn't mine any 
blocks on top of $B_i$. State $(1,1)$ corresponds to the 
state where adversary releases its one length hidden chain to
compete against the block mined by the honest miners.
Transitions in the state corresponds to block mining 
events either by the honest miners or by the adversary himself. 

\begin{figure}[!h]
\centering
\includegraphics[width=0.9\linewidth]{images/hca-mc.pdf}
\caption{Markov Chain used in computing the fraction of late blocks
in Hidden Chain Attack for both Reset After Release and Mine After
Release adversarial strategy.}
\label{fig:hidden chain mc}
\end{figure}

Let $\lambda=\alpha+\beta$. For each state $(x,y)$ with 
$0<x<y-2$, state transition to $(x+1,y)$ and $(x,y+1)$ happens with 
probability $p=\alpha/\lambda$ and $q=\beta/\lambda$ respectively. 
The former corresponds to a new block by the honest miners and the later
implies that \adv mined a new block in its hidden chain.
In both RAR and MAR, \adv releases its hidden chain in the following
situations:
(\romannumeral1)~If \adv's hidden chain contains only one block 
and honest miners mine a competing block at the same height, 
in the MC this corresponds to the state transition form $(0,1)$
to $(1,1)$ which happens with probability $p$; 
(\romannumeral2)~If \adv's hidden chain contains $y>1$ blocks 
and honest miner creates $y-1$ blocks extending $B_i$, it is 
shown by the transition from $(y-2,y)$ to the $(0,j)$ for 
$j\ge0$. We denote the transition probability of such transition 
using $R_{y,j}$. The significance of $j$ will be explained subsequently. 

In the case of (i), once \adv releases its hidden chain, \adv starts
mining on top of its own block to create the next block.
%This is
%because if the \adv mines the next block, \adv will earn two
%block rewards. Also,
Let us assume that $\omega$ fraction of 
the honest miners decides to extend the block mined by the honest
miners and $(1-\omega)$ tries to mine on \adv's block.
%\vinay{Why are we talking about block rewards? Are we plotting those?}
Hence during transition from $(1,1)$ to $(0,0)$, \adv will
get two consecutive blocks in the chain with probability $q$, one block
with probability $(1-\omega)p$ and zero blocks with 
$\omega p$. 

To count the number of late blocks we assume that 
\adv introduces late blocks by releasing the hidden chain only
when $y>\ths$ at the time of release. Hence for both
RAR and MAR:
\begin{equation*}
    R_{y,j} = 
   \begin{dcases}
    1 & \text{if } j=0 \land y\le \ths \\
    0 & \text{if } j>0 \land y\le \ths \\
  \end{dcases}
\end{equation*}

\vspace{1mm}
\noindent{\bf Late blocks in RAR.}
For every release of $y>\ths$, \adv will introduce $y-\ths$ 
late blocks. As a result honest miners will waste their mining 
power for the next $(A_{\advi}(t)-\ths+1)\tau$ units of time. 
In RAR, \adv utilizes this interval to mine blocks for the 
next cycle of the attack. So, if adversary mines $j$ blocks 
in the time interval $(y-\ths+1)/\tau$, this corresponds to 
the state transition from $(y-2,y)$ to $(0,j)$. This happens 
with probability
\begin{equation}
R_{y,j} = p\frac{(\beta(y-\ths+1)\tau)^je^{-\beta(y-\ths+1)\tau}}{j!}
\label{eq:hca reset}
\end{equation}
and the number of late blocks in such transition is $(y-\ths)$.

\vspace{1mm}
\noindent{\bf Late blocks in MAR.}
Similar to RAR, if \adv releases a hidden chain of length 
$y>\ths$ in MAR, honest miners will waste their mining power for next
$(y-\ths+1)\tau$ units of time. Let $N_0 = A_{\advi}(t)-\ths$
and we refer to the time interval $(y-\ths+1)\tau$ as 
the {\em first silent} period. Let $N_1$ be the random
variable denoting the number of additional blocks \adv mines
in the first silent period. This will extend the silent 
period by $N_1\tau$ units of time. We refer to this increase 
as the second silent period and so on. Generalizing the 
above, let $N_j$ be the random variable denoting the number of 
blocks mined during the $j^{\rm th}$ silent period, then the attack 
lasts till $N_i$ is $0$ for some particular $i$. The event $N_i=0$
implies that the honest queue will be equal to $\ths$ after
the $i^{\rm th}$ silent period. As a result \adv\ will restart 
its attack on top of the latest known block. Observe that, 
by following the above-mentioned strategy on every such release, the
adversary will add to the chain $A_{\advi}(t)+N_1+N_2+\cdots+N_{i-1}$ 
blocks of its own of which $N_0+N_1+\cdots+N_{i-1}$ blocks 
are late. Also since in MAR, \adv always transitions to state
$(0,0)$, $R_{j,y}=1$ for $j=0$ and is equal to zero for $j>0$.

\vspace{1mm}
\noindent{\bf Stationary Probability.}
With the MCs described above, we compute the 
(\romannumeral1) the fraction of late blocks, and (\romannumeral2)
the fraction of blocks mined by the adversary by first evaluating
the stationary probabilities $\Psi=\{\psi_i\}$ for each state $i$. 
To compute the stationary probabilities we truncate the MC
at some $y=M$ for large $M$ ($M>\ths$) and add transitions from states 
$(x,M)$ with $x<M-1$ to $(0,j)$ with probability $R_{j,M}$.
This is equivalent to a strategy where once \adv mines
$M$ blocks in its hidden chain, it does not wait for the honest
miners to catch up and immediately releases its chain.
%before honest miners
%could mine $M-2$ blocks, on mining the $(M+1)^{\rm th}$ block, 
%\adv releases all block from its hidden chain and restarts
%the attack.
This modification converts the MC into a finite MC 
with one recurrent class where all states are positive recurrent. 
This implies that the modified MC is ergodic and a unique 
stationary distribution 
exists~(Thm. 7.7 ~\cite{mitzenmacher2017probability}).

For any given choice of
$\ths,\tau,\alpha,\beta,\omega$ and $M$, we
numerically compute the stationary probabilities $\Psi=\{\psi(i)\}$
for each state $i$.
Let $X(i,j)$ and $Y(i,j)$ denote the expected number of late and 
total blocks respectively during the transition from state $i$ to 
state $j$. Since the MC is ergodic, the fraction of late blocks 
after $m$ state transitions converges in probability as  
$m\rightarrow \infty$ to
\begin{equation}
    \frac{\sum_i \psi(i) \sum_{\forall j} X(i,j){\rm Pr}[i \rightarrow j]}{\sum_i \psi(i) \sum_{\forall j} Y(i,j){\rm Pr}[i \rightarrow j]}
\end{equation}
%, then number of late
%blocks for each state $i$ given by $X(i)$ is:
%%
%\begin{equation}
%    X(i) = \sum_{\forall j} \psi(i)X(i,j){\rm Pr}[i
%    \rightarrow j]
%\end{equation}

%\noindent Hence the total number of late blocks $X$ in the attack
%is:
%\begin{equation}
%    X = \sum_{\forall i} X(i)
%\end{equation}

%Notice that for each release of the hidden chain in RAR, the exact 
%count of late blocks is known. But late blocks in MAR 
%are random variables.
\noindent{\bf Remark:} In our analysis of MAR we count the 
expected number of late blocks as $N_0+\sum_{j=1}^i E[N_j]$.
Also, we use the same approach while counting the total
expected number of blocks that appear in the final blockchain.
Figure~\ref{fig:hca compare} compares our theoretical
results with results obtained from discrete event simulation.
