# Supplementary material for: Better Late than Never; Scaling Computation in Blockchains by Delaying Execution
Source: arXiv:2005.11791 source file (2021-06-02)
Supplement: Supplementary file 2 [file thm-proof.tex]

% !TEX root = ../main.tex
\section{Proof of Theorem~\ref{thm:queue size}}
\label{apx:queue size pf}
\section{Proof of Theorem~\ref{thm:OCA}}
\begin{proof}
Now let us analyze the queue of an honest miner during the OCA attack.
Here when the queue size is less than $\ths$ the input rate is
$\lambda=\alpha+\beta$, otherwise it is merely
$\beta$. We can form any input realization for this queue by
starting from an input realization of the \md1 queue and remove the
honest blocks in certain periods.  As a consequence, it follows that
the probability of this queue exceeding $\ths-1$ is smaller 
than that of the \md1 queue, which is upper bounded by $\epsilon_0$.

Now the attacker's blocks are a Poisson process. Hence the 
PASTA property applies to them. Hence the fraction of 
attacker's blocks which see a queue of size $\ths$ or high
is less than $\epsilon_0$. Also as we assume, no honest ES-block end 
up in the blockchain, the fraction of blocks \adv\ mines during
an overflowing queue is upper bounded by $\epsilon_0$.
\end{proof}
\noindent
{\bf Remark}
In the proof above, we have used that \md1 queuing system adheres 
to the Poisson Arrival See Time Average~(PASTA)~\cite{wolff1982poisson} rule.
PASTA states that the probability that a block on arrival will 
find $l$ blocks in the queue is same as $\pi_l$. Hence, the fraction 
of late blocks i.e. blocks which on arrival will see a queue of 
size or $\ths$ or more in the above \md1 process will be 
bounded above by $\epsilon_0$ using equation~(\ref{eq:md1 bound}). 
%
%However since the input rate $\lambda$ in \prot\ does is not fixed 
%throughout, $\pi_l$ in equation~(\ref{eq:md1 general}) is not 
%equal to probability of queue size being $l$ in \prot. 
%But notice that the input rate $I_t$ at $\queue$ is upper 
%bounded by $\lambda_{\hsti} + \lambda_{\advi}$ for all time $t$. Hence
%for a given security threshold $\beta$, $\ths^*$ computed 
%using equation~(\ref{eq:md1 bound}) with 
%$\lambda=\lambda_{\hsti}+\lambda_{\advi}$ will upper bound the fraction
%of late blocks in \prot\ as well.
