# Supplementary material for: Better Late than Never; Scaling Computation in Blockchains by Delaying Execution
Source: arXiv:2005.11791 source file (2021-06-02)
Supplement: Supplementary file 3 [file appendix.tex]

% !TEX root = ../main.tex

%This approach is correct as the considered Markov chain
%is ergodic. Using the same approach, we also compute the 
%total number of blocks that become part of the blockchain 
%using the same Markov chain. Using this total count, we 
%compute the fraction of late blocks.


% \subsection{Confirmation Time}
% \begin{definition}
% (Confirmation Time) The confirmation time is the minimum depth that a block must be in the chain of an honest miner to ensure
%   that it cannot be removed 
%   with probability higher than a specified security parameter
%   by an adversary mining a hidden chain
% \end{definition}

% Since in \prot\ honest miners may temporarily stop mining for a short 
% duration, consistency results first proved by Pass et al. 
% in~\cite{pass2017analysis} and later improved by Kiffer et al. 
% are not directly applicable here. These proofs assume that 
% the honest miners mine for the entire duration of the protocol
% hence can be applied only till queue of the honest miners
% reaches $\ths^*+1$ for the first time. 
% Hence we only focus on confirmation time (in number of blocks)
% for the transactions that enter the blockchain and demonstrate
% that it does not differ from standard PoW blockchains using
% discrete event simulation. We first theoretically compute
% the success probability of an adversary \adv\ trying to double
% spend in standard PoW blockchains 
% from~\cite{rosenfeld2014analysis}. Note that we do not directly
% use their results and add a correction term whose rationale in 
% given in Appendix~\ref{apx:rosenfeld correction}. We then 
% simulate the double-spend attacks in \prot\ using a discrete 
% event simulator for various $\ths^*$ and fraction of mining 
% power controlled by the attacker. 

% With $n$ as the confirmation time, in our simulations
% %to double-spend a transaction from a block $B_i$,
% \adv secretly forks 
% from the parent block $B_i$ immediately after its creation. 
% After $B_i$ gets $n$ confirmations in the honest chain, if \adv's hidden chain is
% longer, \adv continues to extend its hidden chain till 
% honest miners catch up to one block behind. Once honest miners
% catch up, \adv releases its hidden chain and successfully performs the double spend. The intuition for doing so rather than immediately release its hidden chain  after $n$ confirmations is the following.
% Using the notation of our analysis, assume that $Q_t=L_t$ at the time the hidden chain is released and that this becomes the starting queue size for the next attack. A larger starting queue size 
% increases the chances of non-mining periods during the next attack and hence its success probability. Hence waiting for the honest miners to catch up maximizes $L_t$ which maximizes 
% the success probability of the next attack.


% Alternatively, when honest miners have
% a longer chain than the adversary, \adv continue to mine till 
% honest miners are ahead by $r'$ blocks. At this point, \adv 
% gives up and restarts the attack at the end of the honest chain. 
% Figure~\ref{fig:ds prob} compares our simulation results with
% the theoretical ones computed using equation~(\ref{eq:rosen correction}).
% %
% \pgfplotsset{small,label style={font=\fontsize{8}{9}\selectfont},legend style={font=\fontsize{7}{8}\selectfont},height=4.5cm,width=0.9\linewidth}
% \begin{figure}[h!]
%     \centering
%     % \pgfplotsset{footnotesize,height=5cm, width=0.90\linewidth}
%     \begin{tikzpicture}
%     % \begin{axis}
%     \begin{semilogyaxis}
%     [
%         legend pos=south west,
%         legend columns=2,
%         xlabel={Number of Confirmations},
%         ylabel= {Double Spend Probability},
%         grid=none,
%         ]
%         \addplot [red, solid, mark=*, mark size=0.5pt, error bars/.cd, y explicit, y dir=both,] 
%         table [x=constTh, y=k15, y error=cfi15, col sep=comma] {data/sim-res-dst.csv};
%         \addplot [orange, solid, mark=*, error bars/.cd, y explicit,y dir=both,] 
%         table [x=constTh, y=k25, y error=cfi25, col sep=comma] {data/sim-res-dst.csv}; 
%         \addplot [red, dashed, mark options=solid, mark=o,mark size=0.5pt,]
%         table [x=constTh, y=k35, y error=cfi35, col sep=comma] {data/sim-res-dst.csv};
%         % \addplot [black,  mark=+,] 
%         % table [x=constTh, y=k45, y error=cfi45, col sep=comma] {data/sim-res-dst.csv}; 
%         % \addplot [red, dashed, mark options=solid, mark=o,mark size=0.5pt,]
%         % table [x=constTh, y=k55, y error=cfi55, col sep=comma] {data/sim-res-dst.csv};
%         % \addplot [red, mark=diamond,]
%         % table [x=constTh, y=k65, y error=cfi65, col sep=comma] {data/sim-res-dst.csv};

%         \addplot [blue, dashed, mark options=solid, mark=x,] 
%         table [x=queueLen, y=theoDst, col sep=comma] {data/theo-res-dst.csv}; 
%         \addlegendentry{$\ths=15$}
%         \addlegendentry{$\ths=25$}
%         \addlegendentry{$\ths=35$}
%         % \addlegendentry{$\lambda=45$}
%         % \addlegendentry{$\lambda=55$}
%         % \addlegendentry{$\lambda=65$}
%         \addlegendentry{Theoretical}
%     \end{semilogyaxis}
%     % \end{axis}
%     \end{tikzpicture}
%     \caption{Success probability of a double spend attack by 
%     a adversary (\adv) controlling $f=0.33$ of the mining power
%     with varying number of confirmation blocks for different 
%     $\ths^*$. In all attacks, \adv restarts the 
%     attack if honest miners are 64 blocks ahead of him i.e $r'=64$.
%     These probabilities are computed using a 
%     discrete event simulation where for $\ths^*$ and 
%     confirmation time, we simulated 1 Million attack events 
%     and computed the the number of time \adv succeeds 
%     in the attack. This corresponds to a blockchain of 130 
%     Million blocks. All numbers are averaged over 10 runs. 
%     Theoretical results are computed for standard Nakamoto 
%     consensus computed with probability expression given in 
%     Appendix~\ref{apx:rosenfeld correction}.}
%     \label{fig:ds prob}
% \end{figure}

% \subsection{Difficulty Adjustments}
% \label{sub:diff adjustments}
% The purpose of all {\em Difficulty Adjustments Algorithm}~(DAA)
% in blockchains to keep a fixed average interarrival 
% time~$(\Delta)$ between blocks on the face of varying mining 
% power. In the absence of DAA, an increase in mining power of 
% the network will reduce $\Delta$ and vice-versa. Since lower
% $\Delta$ can increase the fraction of late blocks in \prot\ we 
% are interested in \prot's behavior in the presence of a Byzantine
% adversary and DAA.
% Throughout this discussion, we consider a
% DAA of adjusting the puzzle difficulty after every fixed number of blocks $M$ for large $M$. 

% We consider the scenario where any attack begins just after a
% difficulty adjustment and then continues thereafter. We make the
% approximation that the average rate of blocks entering the chain
% between two difficulty adjustments is equal to the long-term ergodic
% mean rate achieved when $M\rightarrow \infty$. Before the attack
% begins, the average block rate entering the chain is $\lambda_{\hsti}$, the block arrival rate in the presence of no adversary. After the next adjustment it is again the same and remains so thereafter. We wish to know how the attack performs in the period before the first adjustment (period-1) and also thereafter (period-2).

% \begin{theorem}
%   Assume that for the OCA attack $\ths^*$ is chosen to ensure  security parameter $\beta$. Then in both period-1 and period-2 the fraction of late blocks is less than $\beta$.
%     The same result holds for the  HCA attacks.
% \end{theorem}
% \begin{proof}
% First let us analyze OCA.
% Suppose $\ths^*$ is chosen according to
% equation~\ref{eq:md1 bound} with
% $\lambda=\lambda_{\hsti}+\lambda_{\advi}$.
% %then \adv\ will not be able
% %to  increase block arrival rate using either OCA or the
% %two HCA attacks.
% Then during period-1, the fraction of late blocks is less than $\beta$ according to Therorem \ref{thm:OCA}.
% In period-1, the
% chain grows at rate $\lambda$ which reduces to 
% to $\lambda_{\hsti}$ in period-2. Hence the fraction of late blocks is even lower than in period-1.

% %This is because to reduce the puzzle difficulty, \adv needs to ensure
% %that the system as a whole generates blocks at a lower rate where as
% %in OCA, \adv increases the block generation rate instead. Hence
% %difficulty adjustment will in fact mitigate OCA once the attack
% %starts.

% In HCA consider period-1.
% Suppose $\ths^*$ is chosen according to
% Figure \ref{fig:hca compare} so that the fraction of late blocks is less than security parameter $\beta$. This ensures by design, that in period-1 the fraction of late blocks is less than $\beta$.
% Note that in period-1, \adv\ replaces honest blocks by more blocks of its own.
% Hence,
% neglecting the time for which honest miners do not mine (which we have
% demonstrated can be made arbitrarily small), the rate at which blocks
% are added to the chain is larger than $\lambda_{\hsti}$.
% In period-2, similar to the OCA attack, the block rate slows down to $\lambda_{\hsti}$. Hence the fraction of late blocks is less than in period-1.
% \end{proof}




% \subsection{Gas Limit vs Gas Usage}
% \label{apx:gas usage}
% Using historical Ethereum block chain data we measure how well 
% Ethereum users predict gas usage for contract transactions. 
% Figure~\ref{fig:gas usage} illustrates our findings.
% Observe that


% In this paper we only derive transaction probabilities for 
% $c>1/2$ as one can easily derive for $c\le1/2$ using similar
% approach.

% As being in state $1$ represents that the last block was
% mined by node $n_1$ at time $t=0$, all miners except 
% $n_1$ will validate the block till time $\tau$ and will
% create the next block in the interval $(\tau,2\tau]$. As
% $n_1$ takes only $c\tau$ units of time to create
% the next block, $n_1$ will start mining the block at
% time $c\tau$. Hence in the interval $(c\tau,2\tau]$ only
% $n_1$ will be mining. Diagram in the top of 
% Figure~\ref{fig:eth honest timing} these information. In the
% Figure $\emptyset$ during the interval $(0,c\tau]$ implies
% that no miners will do PoW during this period. Also $N$
% in the figure refers to set of all miners.

% Similarly when the last block was mined by a miner other than
% $n_1$, no miner will start PoW till $\tau$ units of time. 
% Say $n_i$ with $i\ne1$ mined the last block, then during time 
% interval $(\tau,2c\tau]$ only $n_i$ will be mining the block
% as $n_1$ will be busy forming the next block during this 
% interval. Once $n_1$ finishes forming the next block, $n_1$
% will start PoW at time $2c\tau$ while others miners will
% start only at time $2\tau$. 

% \begin{figure*}[!htb]
% \centering
% \minipage{0.65\textwidth}
%     \pgfplotsset{label style={font=\fontsize{8}{9}\selectfont},height=4cm,legend style={font=\fontsize{7}{8}\selectfont},width=1.1\linewidth,compat=1.9}
% \begin{subfigure}{0.35\linewidth}
%     \centering
%     \begin{tikzpicture}
%     \begin{axis}[
%         ybar,
%         enlargelimits=0.25,
%         bar width=5pt,
%         /pgfplots/ybar=0pt,
%         legend columns=2,
%         xlabel={$\tau/\Delta$},
%         symbolic x coords={12, 120, 240},
%         grid=minor,
%         xtick={12, 120, 240},
%         ymin=55,
%         ymax=105,
%         ]
%         \addplot [pattern = north east lines] [error bars/.cd, y explicit,y dir=both,] table [x=gasUsage, y=frac1, y error=cfi1, col sep=comma] {data/evd-minefrac.csv}; 
%         \addplot [fill=red!30!white] [error bars/.cd, y explicit,y dir=both,] table [x=gasUsage, y=frac1,y error=cfi2, col sep=comma] {data/evd-minefrac-skip.csv};
%         \addplot [pattern = north east lines] [error bars/.cd, y explicit,y dir=both,] table [x=gasUsage, y=frac2, y error=cfi2, col sep=comma] {data/evd-minefrac.csv};
%         \addplot [fill=red!30!white] [error bars/.cd, y explicit,y dir=both,] table [x=gasUsage, y=frac2,y error=cfi2, col sep=comma] {data/evd-minefrac-skip.csv};
%         \addplot [pattern = north east lines] [error bars/.cd, y explicit,y dir=both,] table [x=gasUsage, y=frac3, y error=cfi3, col sep=comma] {data/evd-minefrac.csv};
%         \addplot [fill=red!30!white] [error bars/.cd, y explicit,y dir=both,] table [x=gasUsage, y=frac3,y error=cfi3, col sep=comma] {data/evd-minefrac-skip.csv};
%     \end{axis}
%     \end{tikzpicture}
%     \caption{\prot, $\Delta=\frac{1}{\lambda}=15,\delta=1$}
%     \label{fig:tuxedo high tau}
%     \end{subfigure}
%     %
%     \begin{subfigure}{0.30\linewidth}
%     \centering
%     \begin{tikzpicture}
%     \begin{axis}[
%         ybar,
%         enlargelimits=0.25,
%         bar width=5pt,
%         /pgfplots/ybar=0pt,
%         legend columns=2,
%         xlabel={$\delta$},
%         symbolic x coords={1.0,2.0,4.0},
%         xtick={1.0,2.0,4.0},
%         grid=minor,
%         ymin=55,
%         ymax=105,
%         ]
%         \addplot [pattern = north east lines] [error bars/.cd, y explicit,y dir=both,] table [x=delay, y=frac1, y error=cfi1, col sep=comma] {data/evd-minefrac-delay.csv}; 
%         \addplot [fill=red!30!white] [error bars/.cd, y explicit,y dir=both,] table [x=delay, y=frac1,y error=cfi1, col sep=comma] {data/evd-minefrac-delay-skip.csv};
%         \addplot [pattern = north east lines] [error bars/.cd, y explicit,y dir=both,] table [x=delay, y=frac2, y error=cfi2, col sep=comma] {data/evd-minefrac-delay.csv};  
%         \addplot [fill=red!30!white] [error bars/.cd, y explicit,y dir=both,] table [x=delay, y=frac2,y error=cfi2, col sep=comma] {data/evd-minefrac-delay-skip.csv}; 
%         \addplot [pattern = north east lines] [error bars/.cd, y explicit,y dir=both,] table [x=delay, y=frac3, y error=cfi3, col sep=comma] {data/evd-minefrac-delay.csv};  
%         \addplot [fill=red!30!white] [error bars/.cd, y explicit,y dir=both,] table [x=delay, y=frac3,y error=cfi3, col sep=comma] {data/evd-minefrac-delay-skip.csv}; 
%         % \addlegendentry{Honest}
%         % \addlegendentry{Adversarial}
%     \end{axis}
%     \end{tikzpicture}
%     \caption{\prot, $\frac{\tau}{\Delta}=0.74,\ths=50$}
%     \label{fig:tuxedo high delay}
%     \end{subfigure}
% \endminipage\hfill
% %
% \minipage{0.35\textwidth}
%     \pgfplotsset{label style={font=\fontsize{8}{9}\selectfont},height=4cm,legend style={font=\fontsize{7}{8}\selectfont},width=\linewidth}
%     \begin{tikzpicture}
%     \begin{axis}[
%         legend pos=north east,
%         xlabel={block height (Millions)},
%         ylabel= {bas Usage (Millions)},
%         ytick=\empty,
%         extra y ticks={4000000,6000000,8000000},
%         extra y tick labels = {4,6,8},
%         xtick=\empty,
%         extra x ticks={5000000,5050000,5100000,5150000,5200000,5250000,5300000},
%         extra x tick labels = {5.00,5.05,5.10,5.15,5.20,5.25,5.30},
%         grid=minor,
%         legend columns=2,
%         ymax=9000000,
%         ]
%         \addplot[mark=square, black] table [x=blockHeight, y=gasUsedEthereum, col sep=comma] {data/percentOfContractTransFract.csv}; 
%         \addplot[mark=+, blue] table [x=blockHeight, y=gasUsedEVD, col sep=comma] {data/percentOfContractTransFract.csv};
%         \addlegendentry{Ethereum}
%         \addlegendentry{Tuxedo}
%     \end{axis}
%     \end{tikzpicture}
%     \caption{Gas usage in \prot\ for Ethereum blocks in the 
%     range 5M to 5.3M}
%   \label{fig:gas compare}
% \endminipage\hfill
% \end{figure*}
